# Supplementary material for: Hardware Resilience Properties of Text-Guided Image Classifiers
Source: arXiv:2311.14062 source file (2023-12-05)
Supplement: Supplementary file 1 [file main_supp.tex]

\begin{table}[ht]
\centering
\caption{The tables present results across various backbones, reporting top-1 accuracy on the ImageNet validation set for both the baseline and our method. Additionally, we report the improvment in last-layer and overall model reliability, and a percentage increase in Top2Diff.}
\scalebox{0.90}[0.90]{
\begin{tabular}{lccccccc}
    \toprule
    Backbone   & \begin{tabular}[c]{@{}c@{}}Acc.\\ Baseline\end{tabular} & \begin{tabular}[c]{@{}c@{}}Acc.\\ Ours\end{tabular} & \begin{tabular}[c]{@{}c@{}}Improvement\\ in Reliability\\ (Last Layer)\end{tabular} & \begin{tabular}[c]{@{}c@{}}Improvement\\ in Reliability\\ (Overall)\end{tabular} & \begin{tabular}[c]{@{}c@{}}Improvement\\ in Top2Diff\end{tabular}\\
    \midrule
    Alexnet         & $56.43$    &    $57.28$    &    $7.92\times$     &    $4.67\times$    &    $2.83\%$ \\
    MobileNet-V2    & $71.87$    &    $71.83$    &    $3.92\times$     &    $2.43\times$    &    $5.36\%$ \\
    Swin-V2-T     & $80.97$    &    $81.02$    &    $1.65\times$     &    $1.07\times$    &    $2.85\%$ \\
    \bottomrule
\end{tabular}}
\label{tab:main_supp}
% \vspace{-.4cm}
\end{table}
